# Supplementary material for: Schr\"odinger cat states of a nuclear spin qudit in silicon
Source: arXiv:2405.15494 source file (2025-01-14)

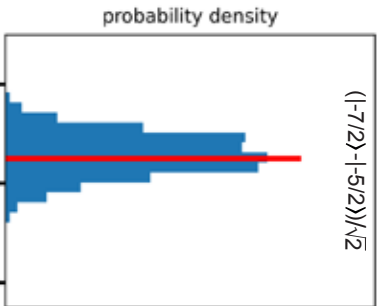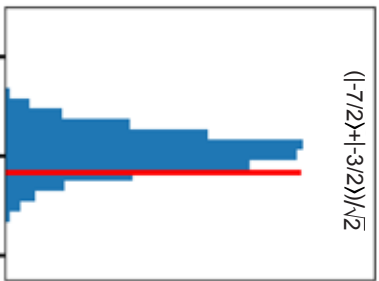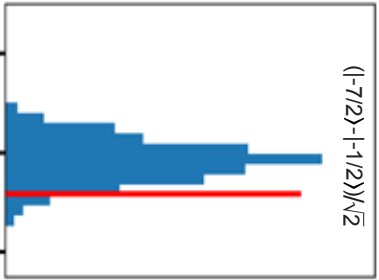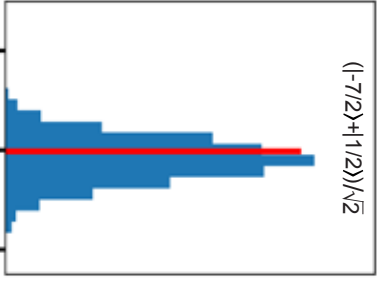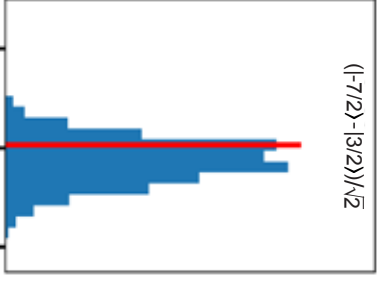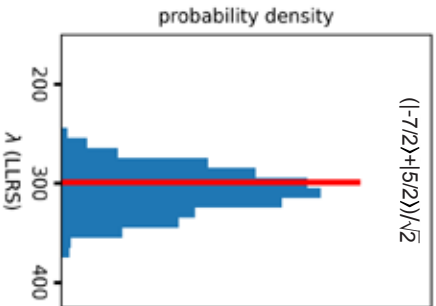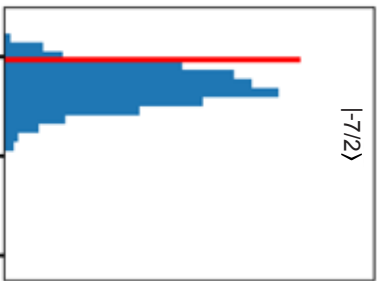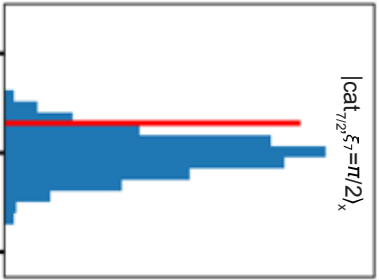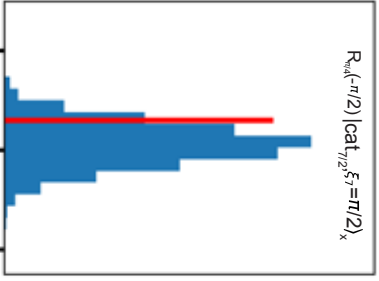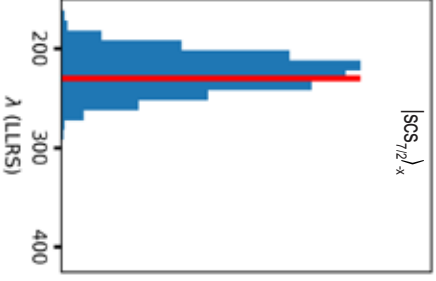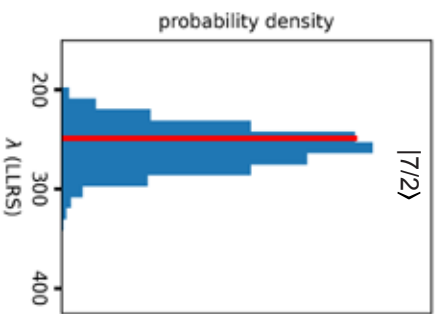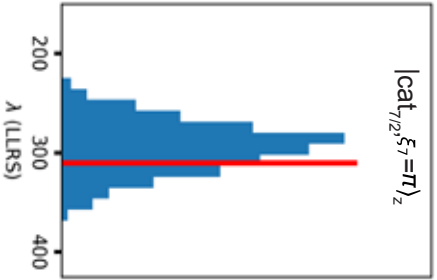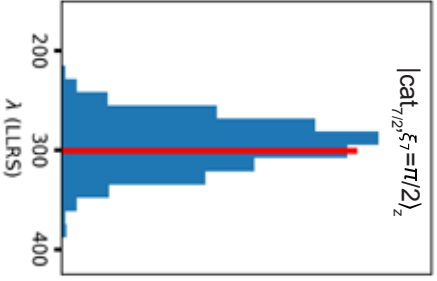

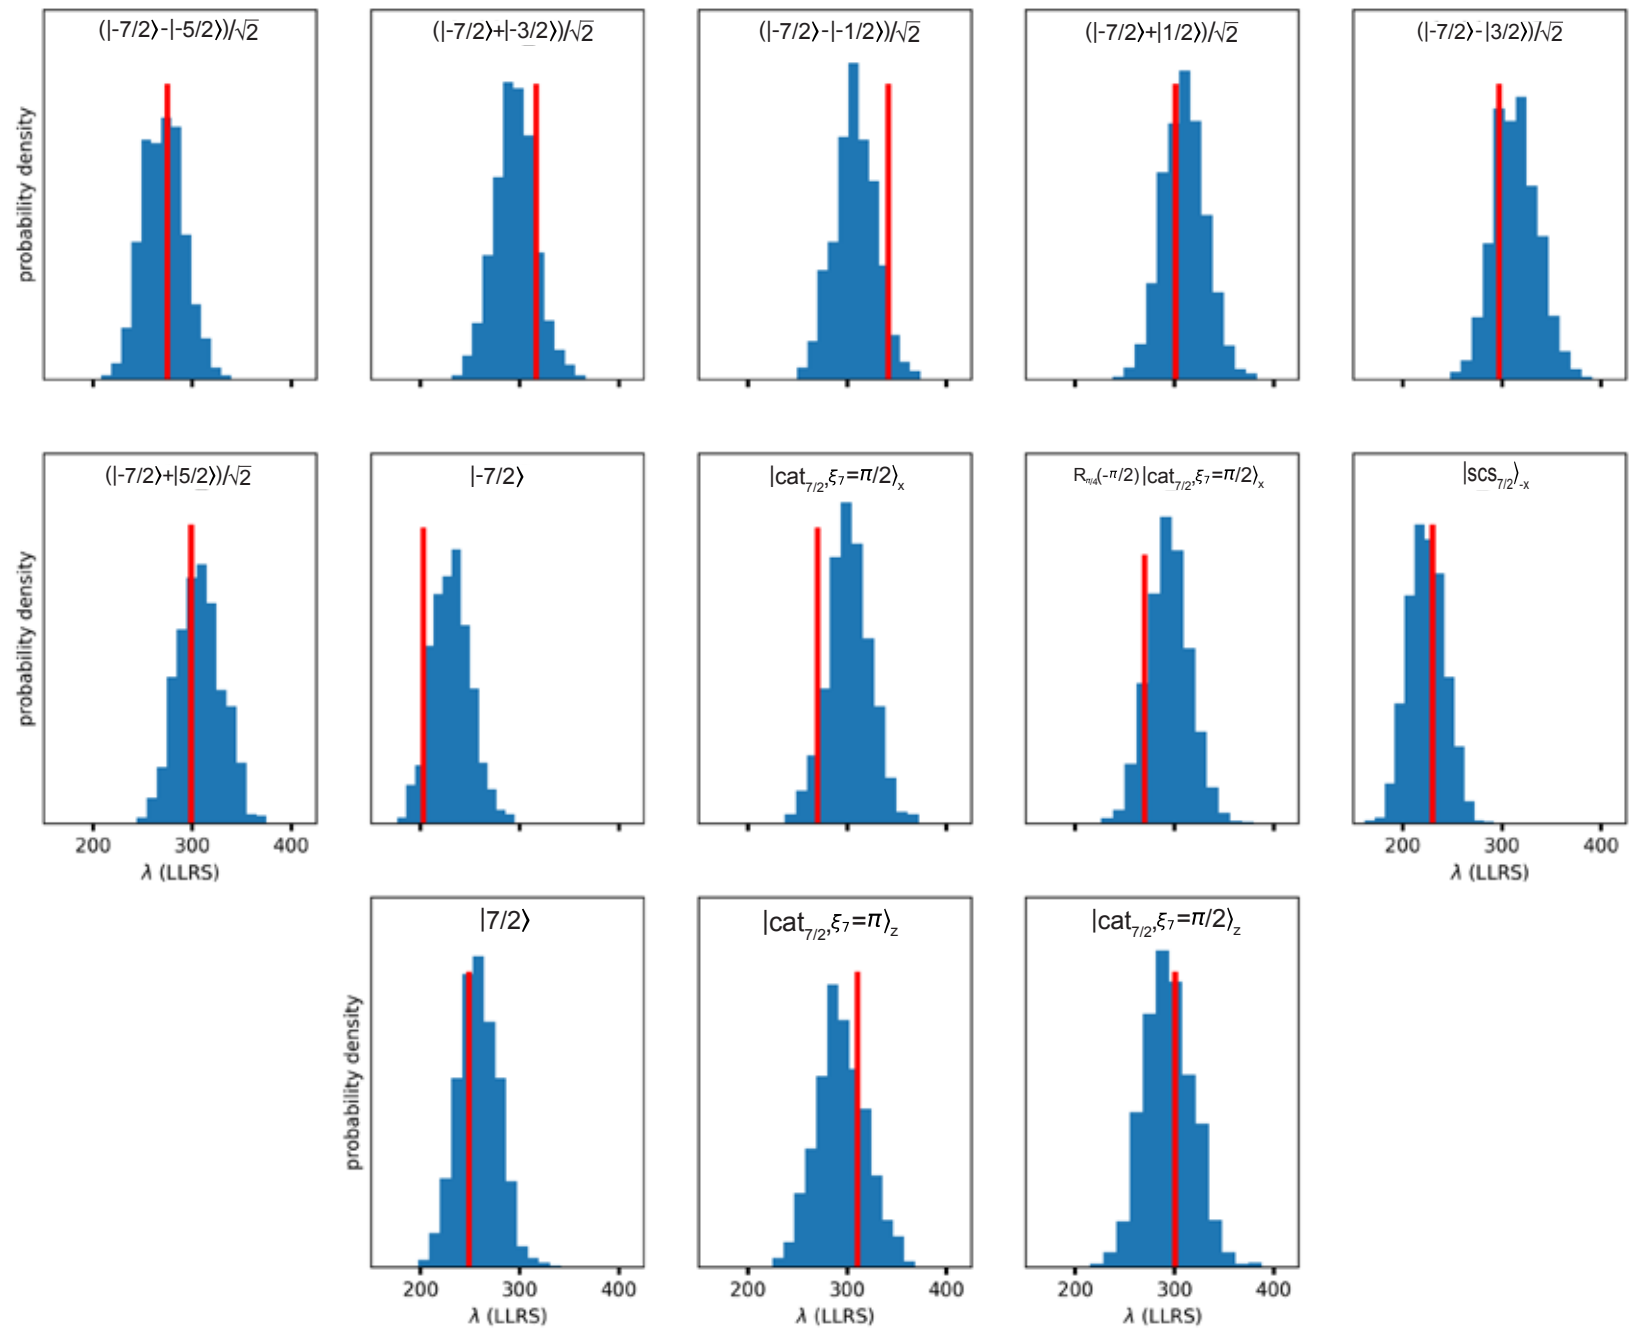

Supplement: Supplementary file 1 [file TomographyValidation.pdf]
